# Supplementary material for: Benchmarking and Error Diagnosis in Multi-Instance Pose Estimation
Source: arXiv:1707.05388 source file (2017-08-05)
Supplement: Supplementary file 2 [file 6_appendix.tex]

\section{Correction of Localization Errors}
\label{subsec:error_correction}
\setcounter{figure}{0}

The fine-grained PR curves shown in Fig.~\ref{fig:intro_supp_123} are obtained by fixing an OKS threshold and evaluating the performance of an algorithm after progressively correcting its detections. To do so, we compute for every predicted keypoint what is the Keypoint Similarity (KS) with its corresponding ground-truth body part, and with different ground-truth body parts of the same person, and of all other people contained in the image. This allows us to identify the types of localization error, as done in Sec. 3.1, and correct them. %We indicate with $\mathbf{\hat{\theta}}_i^{(p)}$ and $\mathbf{\theta}_i^{*,(p)}$ respectively the predicted and corrected location for keypoint $i$ of a detection, and with $\mathbf{\theta}_j^{(p)}$ the ground-truth location for keypoint $j$ of the annotation of a person $p$.\\

\begin{itemize}

\item \textbf{Miss} errors are corrected by repositioning a keypoint prediction on the .5 KS circle centered on the true location; \textit{left-elbow} and \textit{wrists} in Fig.~\ref{fig:error_correction}.

\item \textbf{Swap} and \textbf{Inversion} errors are corrected by repositioning a keypoint prediction at a distance from the correct ground-truth location so that the new value of KS is the same that the prediction had with the wrong body part it mistakenly detected (belonging to a different/same person for swap/inversion); \textit{E.g}.: in Fig.~\ref{fig:error_correction}.(Top) the \textit{right-elbow} has a swap error with the, while the \textit{right-knee} has an inversion error.

\item \textbf{Jitter} errors are corrected by repositioning a keypoint prediction on the .85 KS circle centered on the true location; \textit{left-ankle} in Fig.~\ref{fig:error_correction}.

\end{itemize}

\textit{Miss} and \textit{jitter} errors are corrected by bringing a prediction to a fixed distance from its true position. The new location of \textit{swaps} and \textit{inversions} instead depends on how good was the prediction of the wrong joint: after correction, a good/bad prediction of the wrong body part becomes a good/bad prediction (high/low KS) of the true body part. 

Fig.~\ref{fig:error_correction} provides two examples of how the keypoints belonging to a detection can be progressivily improved. The OKS increase obtained by correcting the localization errors depends both on the number of errors of that type, and the total number of visible keypoints present in an instance, see Eq. 1. Fixing the position of predicted keypoints impacts the overall AUC of the PR curves: the detection in Fig.~\ref{fig:error_correction}.(Top), which previously was a FP at OKS evaluation thresholds above .75, after correction has become a TP at all thresholds between .75 and .9.

\begin{figure}[t!]
\centering
\includegraphics[width=\linewidth]{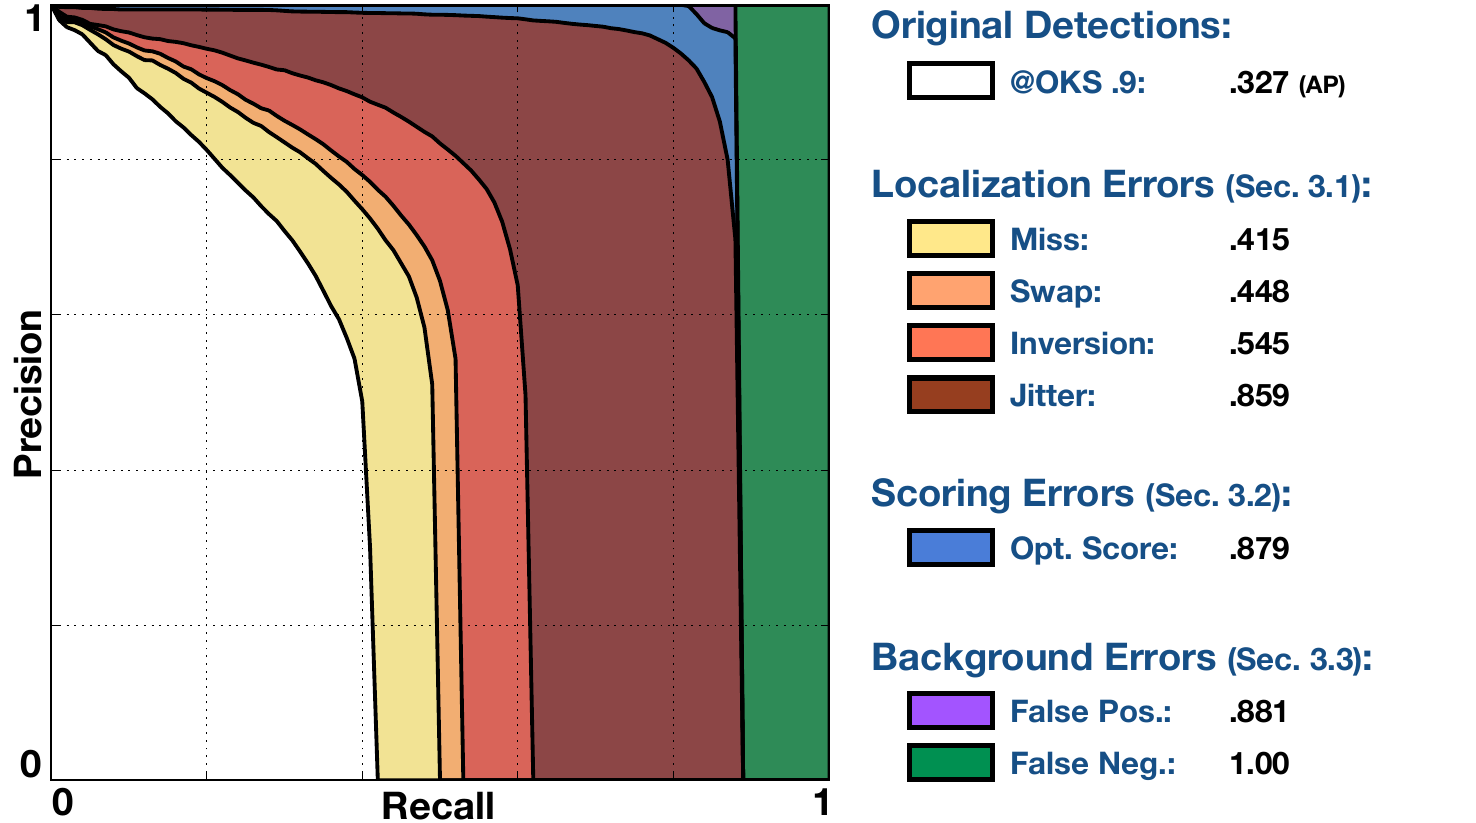}
{\caption {\small \textbf{Coarse to Fine Error Analysis.}}}
\vspace{-5mm}
\label{fig:intro_supp_123}
\end{figure}

\section{Human Pose and Skeleton Color Coding}
\label{subsec:color_coding}

%%%%%%%%%%%%%%%%%%%%%%%%%%%%%%%%%%%%%%%%%%%%%%%%%%%%%%%%%%%%%%%%%%%%%%%%%%%%%%%%%%%%%%%%%%%%%%%%%%%%%%%%%%%%
% FIGURE WITH THE EXAMPLE BREAKDOWN THAT CAN BE OBTAINED WITH NEW TOOLS
\begin{figure}[h!]
\centering
\includegraphics[width=.85\linewidth]{./images/_supp_mat_Figure_2.pdf}
\caption{ {\small \textbf{Human Pose and Skeleton Color Coding.}}}
\label{fig:supp_mat_figure_2}
\vspace{-3mm}
\end{figure}
%%%%%%%%%%%%%%%%%%%%%%%%%%%%%%%%%%%%%%%%%%%%%%%%%%%%%%%%%%%%%%%%%%%%%%%%%%%%%%%%%%%%%%%%%%%%%%%%%%%%%%%%%%%

We adopt the following color coding to visualize algorithm's keypoint detections:
\begin{itemize}
    \item The location of the left and right parts of the body is indicated respectively with red and green dots; the location of the nose is plotted in blue.%following the standard used for vessel and aircraft navigation lights
    \item Face keypoints (\textit{nose}, \textit{eyes}, \textit{ears}) are connected by purple lines.
    \item Upper-body keypoints (\textit{shoulders}, \textit{elbows}, \textit{wrists}) are connected by blue lines.
    \item Torso keypoints (\textit{shoulders}, \textit{hips}) are connected by yellow lines.
    \item Lower-body keypoints (\textit{hips}, \textit{knees}, \textit{ankles}) are connected by brown lines.
\end{itemize}

%%%%%%%%%%%%%%%%%%%%%%%%%%%%%%%%%%%%%%%%%%%%%%%%%%%%%%%%%%%%%%%%%%%%%%%%%%%%%%%%%%%%%%%%%%%%%%%%%%%%%%%%%%%%
% FIGURE WITH THE EXAMPLE BREAKDOWN THAT CAN BE OBTAINED WITH NEW TOOLS
\begin{figure*}[t!]
\centering
\begin{tabular}{c}
\includegraphics[width=\linewidth]{./images/_supp_mat_error_correction.pdf}\\[1.25ex]
\includegraphics[width=\linewidth]{./images/_supp_mat_error_correction_2.pdf}\\[1.25ex]
\end{tabular}
\caption{ {\small \textbf{Correction of Keypoint Localization Errors.} The change of a detection's keypoint positions and the resulting OKS improvement as localization errors are progressively corrected. We plot the ground-truth skeleton in green and the detection using the color coding discussed below. The red concentric circles indicate the .5 and .85 KS threshold as discussed in Fig.2 of the main paper. When visualizing the individual error types, we show the concentric circles around the ground-truth location only for the keypoints that are being corrected.}}
\label{fig:error_correction}
\end{figure*}
%%%%%%%%%%%%%%%%%%%%%%%%%%%%%%%%%%%%%%%%%%%%%%%%%%%%%%%%%%%%%%%%%%%%%%%%%%%%%%%%%%%%%%%%%%%%%%%%%%%%%%%%%%%

\section{Automatically Generated Reports}

We provide the automatically generated reports for four methods from the ECCV 2016 Keypoint Challenge:
\begin{itemize}
    \item CMU
    \item GRMI
    \item MASKRNN9
    \item CALTECH
\end{itemize}
